# Supplementary material for: Rejection via Learning Density Ratios
Source: arXiv:2405.18686 source file (2025-05-08)
Supplement: Supplementary file 1 [file proof-gen-bound-1.tex]

\section{Proof of \cref{thm:gen_bound_1}}
\label{sec:pf_gen_bound_1}

\begin{proof}
    \begin{align*}
        &\kl(\meas{Q}^{\kl}_{\lambda}, \meas{Q}^{\kl}_{\lambda, n}) \\
        &= \int \log \left(\frac{\dmeas{Q}^{\kl}_{\lambda}}{\dmeas{Q}^{\kl}_{\lambda, n}}(x) \right) \dmeas{Q}^{\kl}_{\lambda}(x) \\
        &= \int \left[ \log \left(\frac{\dmeas{P}}{\dmeas{P}_{n}}(x) \right)
        +
        \log \left(\frac{\exp\left(-\frac{\ell(x)}{\lambda}\right)}{\exp\left(-\frac{\ell(x)}{\lambda} \right)}\right)
        +
        \log \left( \frac{\expect_{\meas{P}_{n}}\left[\exp\left(-\frac{\ell(x)}{\lambda}\right)\right]}{\expect_{\meas{P}}\left[\exp\left(-\frac{\ell(x)}{\lambda}\right)\right]} \right)
        \right] \dmeas{Q}^{\kl}_{\lambda}(x) \\
        &= \int \log \left(\frac{\dmeas{P}}{\dmeas{P}_{n}}(x) \right) \dmeas{Q}^{\kl}_{\lambda}(x)
        +
        \log \left( \frac{\expect_{\meas{P}_{n}}\left[\exp\left(-\frac{\ell(x)}{\lambda}\right)\right]}{\expect_{\meas{P}}\left[\exp\left(-\frac{\ell(x)}{\lambda}\right)\right]} \right)
         \\
        &\leq \int \log \left(\frac{\dmeas{P}}{\dmeas{P}_{n}}(x) \right) \dmeas{Q}^{\kl}_{\lambda}(x)
        +
        \left \vert \log \expect_{\meas{P}_{n}}\left[\exp\left(-\frac{\ell(x)}{\lambda}\right)\right] - \log \expect_{\meas{P}}\left[\exp\left(-\frac{\ell(x)}{\lambda}\right)\right] \right \vert
         \\
        &\leq \int \log \left(\frac{\dmeas{P}}{\dmeas{P}_{n}}(x) \right) \dmeas{Q}^{\kl}_{\lambda}(x)
        +
        \exp\left( \frac{B}{\lambda} \right) \cdot \left \vert \expect_{\meas{P}_{n}}\left[\exp\left(-\frac{\ell(x)}{\lambda}\right)\right] - \expect_{\meas{P}}\left[\exp\left(-\frac{\ell(x)}{\lambda}\right)\right] \right \vert
    \end{align*}
    
    Notice that we can bound the following via a concentration inequality:
    \begin{align*}
        \left \vert \expect_{\meas{P}_{n}}\left[\exp\left(-\frac{\ell(x)}{\lambda}\right)\right] - \expect_{\meas{P}}\left[\exp\left(-\frac{\ell(x)}{\lambda}\right)\right] \right \vert.
    \end{align*}
    In particular, we utilize the standard Hoeffding's inequality with Markov's inequality.
    Thus we have, with \( 1 - \epsilon \) probability,
    \begin{align*}
        &\kl(\meas{Q}^{\kl}_{\lambda}, \meas{Q}^{\kl}_{\lambda, n}) \\
        &\leq \int \log \left(\frac{\dmeas{P}}{\dmeas{P}_{n}}(x) \right) \dmeas{Q}^{\kl}_{\lambda}(x)
        +
        \exp\left( \frac{B}{\lambda} \right) \cdot \left(1 - \exp\left( -\frac{B}{\lambda}\right)\right) \cdot \sqrt{\frac{\log \frac{\epsilon}{2}}{2n}}
         \\
        &= \int \log \left(\frac{\dmeas{P}}{\dmeas{P}_{n}}(x) \right) \dmeas{Q}^{\kl}_{\lambda}(x)
        +
        \left(\exp\left( \frac{B}{\lambda} \right) -1 \right) \cdot \sqrt{\frac{\log \frac{\epsilon}{2}}{2n}}
         \\
    \end{align*}
\end{proof}

\section{Proof of \cref{thm:gen_bound_2}}

\begin{proof}
    First we consider:
    \begin{align*}
        &\Lambda(\lambda) - \Lambda_{n}(\lambda) \\
        &= \lambda \cdot \left[
            \left( \log \expect_{\meas{P}}\left[ \exp\left( -\frac{\ell_{\vartheta}(x)}{\lambda} \right) \right] + \varepsilon \right)
            -
            \left( \log \expect_{\meas{P}_{n}}\left[ \exp\left( -\frac{\ell_{\vartheta}(x)}{\lambda} \right) \right] + \varepsilon \right)
        \right] \\
        &= \lambda \cdot \left[
            \log \expect_{\meas{P}}\left[ \exp\left( -\frac{\ell_{\vartheta}(x)}{\lambda} \right) \right]
            -
            \log \expect_{\meas{P}_{n}}\left[ \exp\left( -\frac{\ell_{\vartheta}(x)}{\lambda} \right) \right] 
        \right] \\
        &\leq \lambda \cdot \exp\left( \frac{B}{\lambda} \right)\left[
            \expect_{\meas{P}}\left[ \exp\left( -\frac{\ell_{\vartheta}(x)}{\lambda} \right) \right]
            -
            \expect_{\meas{P}_{n}}\left[ \exp\left( -\frac{\ell_{\vartheta}(x)}{\lambda} \right) \right] 
        \right] \\
    \end{align*}
    
    Noting that log-sum-exp is a contraction, we have
    \begin{align*}
        &\Lambda_n(\lambda) - \Lambda_{n, m}(\lambda) \\
        &= \lambda \cdot \left[
            \left( \log \expect_{\meas{P}_n}\left[ \exp\left( -\frac{\ell_{\vartheta}(x)}{\lambda} \right) \right] + \varepsilon \right)
            -
            \left( \log \expect_{\meas{P}_{n}}\left[ \exp\left( -\frac{\ell_{\vartheta, m}(x)}{\lambda} \right) \right] + \varepsilon \right)
        \right] \\
        &= \lambda \cdot \left[
            \log \expect_{\meas{P}_n}\left[ \exp\left( -\frac{\ell_{\vartheta}(x)}{\lambda} \right) \right]
            -
            \log \expect_{\meas{P}_{n}}\left[ \exp\left( -\frac{\ell_{\vartheta, m}(x)}{\lambda} \right) \right]
        \right] \\
        &\leq \max_{x \in \mathcal{X}} \vert \ell_{\vartheta}(x) - \ell_{\vartheta, n}(x) \vert \\
        &\leq \max_{x \in \mathcal{X}} \left \vert \expect_{\meas{P}(\cdot \mid \X = x)}[L(\Y, h_{\vartheta}(x))] - \expect_{\meas{P}_{m}(\cdot \mid \X = x)}[L(\Y, h_{\vartheta}(x))] \right \vert
    \end{align*}
    
    \todo{We can improve the following (PAC Bayes etc)?}
    
    For fixed \( \lambda \) we have the following bounds holding with probability at least \( (1 - \delta) \):
    \begin{align*}
        &\Lambda(\lambda) - \Lambda_{n,m}(\lambda) \\
        &\leq
        \lambda \cdot \left( 1 - \exp\left( \frac{B}{\lambda} \right) \right) \cdot \sqrt{\frac{\log \frac{2 \cdot ({\vert \mathcal{X} \vert + 1})}{\delta}}{2n}}
        +
        B^{2} \cdot \sqrt{\frac{\log \frac{2\cdot ({\vert \mathcal{X} \vert + 1})}{\delta}}{2m}}
    \end{align*}
    
    First recall the following equivalence:
    \begin{theorem}[Donsker and Varadhan’s Variational Formula~\cite{}]
        For a measurable bounded function \( h \),
        \begin{equation}
            \log \expect_\meas{P} \left[ \exp\left( h(\X) \right) \right] = \sup_{\meas{Q}} \left[ \expect_{\meas{Q}} h(\X) - \kl(\meas{Q}, \meas{P})\right].
        \end{equation}
        Furthermore, the supremum is obtained via the Gibbs distribution of \( h \) \wrt \( \meas{P} \).
    \end{theorem}
    
    Thus utilizing DV, we have:
    \begin{align*}
        &\Lambda_n(\lambda) - \Lambda_{n, m}(\lambda) \\
        &= \lambda \cdot \left[
            \left( \log \expect_{\meas{P}_n}\left[ \exp\left( -\frac{\ell_{\vartheta}(x)}{\lambda} \right) \right] + \varepsilon \right)
            -
            \left( \log \expect_{\meas{P}_{n}}\left[ \exp\left( -\frac{\ell_{\vartheta, m}(x)}{\lambda} \right) \right] + \varepsilon \right)
        \right] \\
        &= \lambda \cdot \left[
            \log \expect_{\meas{P}_n}\left[ \exp\left( -\frac{\ell_{\vartheta}(x)}{\lambda} \right) \right]
            -
            \log \expect_{\meas{P}_{n}}\left[ \exp\left( -\frac{\ell_{\vartheta, m}(x)}{\lambda} \right) \right]
        \right] \\
        &= \lambda \cdot \left( \sup_{\meas{R}} \left\{
        \expect_{\meas{R}}\left[ -\frac{\ell_{\vartheta}(\X)}{\lambda} \right]
        - \kl(\meas{R}, \meas{P_n})
        \right\}
        -
        \sup_{\meas{S}} \left\{
        \expect_{\meas{S}}\left[ -\frac{\ell_{\vartheta, m}(\X)}{\lambda} \right]
        - \kl(\meas{S}, \meas{P_n})
        \right\} \right) \\
        &= \sup_{\meas{R}} \left\{
        \expect_{\meas{R}}\left[ -\ell_{\vartheta}(\X) \right]
        - \kl(\meas{R}, \meas{P_n})
        \right\}
        -
        \sup_{\meas{S}} \left\{
        \expect_{\meas{S}}\left[ -\ell_{\vartheta, m}(\X) \right]
        - \kl(\meas{S}, \meas{P_n})
        \right\} \\
        &= \inf_{\meas{S}} \sup_{\meas{R}} \left\{
        \expect_{\meas{R}}\left[ -\ell_{\vartheta}(\X) \right]
        - \kl(\meas{R}, \meas{P_n})
        -
        \expect_{\meas{S}}\left[ -\ell_{\vartheta, m}(\X) \right]
        + \kl(\meas{S}, \meas{P_n})
        \right\} \\
        &\leq \sup_{\meas{R}} \left\{
        \expect_{\meas{R}}\left[ -\ell_{\vartheta}(\X) \right]
        - \kl(\meas{R}, \meas{P_n})
        -
        \expect_{\meas{R}}\left[ -\ell_{\vartheta, m}(\X) \right]
        + \kl(\meas{R}, \meas{P_n})
        \right\} \\
        &= \sup_{\meas{R}} \left\{
        \expect_{\meas{R}}\left[ -\ell_{\vartheta}(\X) \right]
        -
        \expect_{\meas{R}}\left[ -\ell_{\vartheta, m}(\X) \right]
        \right\} \\
        &= \sup_{\meas{R}} \left\{
        \expect_{\meas{R}}\left[
        \ell_{\vartheta, m}(\X)
        -\ell_{\vartheta}(\X)
        \right]
        \right\} \\
        &= 
        \expect_{\meas{Q}_{\lambda, n}}\left[
        \ell_{\vartheta, m}(\X)
        \right]
        -
        \expect_{\meas{Q}_{\lambda, n}}\left[
        \ell_{\vartheta}(\X)
        \right],
    \end{align*}
    where for the last line we are using the fact that the Gibbs distribution of \( - \ell(x) / \lambda \) \wrt \( \meas{P}_n \) is exactly \( \meas{Q}_{\lambda} \).
    
    Now notice, that we can use a PAC-Bayes bound. We use the prior distribution \( \meas{P}_n \). Note that \( \meas{P}_n \) is data independent where data in our case are samples of \( y \) (given a fixed \( x \)).
    
    One must be careful here by defining a modified loss \( \ell \)
    \begin{equation*}
        \ell_{\vartheta, m}(x) = \frac{1}{m} \sum_{x \in \mathcal{X}} \sum_{i \in [m]} L(y_{x, i}, h_{\vartheta}(x_{i})) \cdot \iver{x = x_{i}}.
    \end{equation*}
    Here we are exploiting our assumption, that our sampled \( y \)'s are generated by sampling the conditionals \( \meas{P}(\Y \mid \X = x) \) for each \( x \) \( m \)-times.
    
    \todo{We are missing a constant here. The current PAC bound only holds for losses in [0,1]. But ours is bounded by B not 1. }
    
    With slight change in the PAC-Bayes proof (McAllester Bound) to incorporate said loss function and our bounded loss function, we get with probability \(1-\delta\)
    \begin{align*}
        &\Lambda_n(\lambda) - \Lambda_{n, m}(\lambda) \\
        &\leq
        \expect_{\meas{Q}_{\lambda, n}}\left[
        \ell_{\vartheta, m}(\X)
        \right]
        -
        \expect_{\meas{Q}_{\lambda, n}}\left[
        \ell_{\vartheta}(\X)
        \right] \\
        &\leq
        B \cdot
        \sqrt{
        \frac{\kl(\meas{Q}_{\lambda, n}, \meas{P}_{n}) + \log \frac{2\sqrt{m}}{\delta}}{2m}
        } \\
        &\leq
        B \cdot
        \sqrt{
        \frac{\varepsilon + \log \frac{2\sqrt{m}}{\delta}}{2m}
        },
    \end{align*}
    where the last line holds from \( \meas{Q}_{\lambda, n} \in B_{\varepsilon}(\meas{P}_n) \).
    
    \todo{Check this last line. It definitely holds true of \( \lambda \) is optimal for the empirical dist. Maybe, we introduce a class of \( \lambda \), then suppose that the optimal is said class. Then we can union bound + bound this with eps.
    
    Otherwise, we can bound the KL to \( B / \lambda \) via Jensen's.
    }
\end{proof}
