# Supplementary material for: Rejection via Learning Density Ratios
Source: arXiv:2405.18686 source file (2025-05-08)
Supplement: Supplementary file 2 [file proof-mirror-update.tex]

\section{Proof of \cref{thm:mirror_update}}
\label{sec:pf_mirror_update}

\begin{proof}
    We consider the following Lagrangian by considering \cref{todo},
    \begin{equation*}
        \mathcal{L}(\meas{Q}; a(\cdot), b)
        =
        \max\left\{ 0, \frac{\rho}{1+\rho} \cdot (D_{\alpha}(\meas{P} : \meas{Q}) - \varepsilon)\right\} + \frac{1}{1+\rho} \left( D_{\alpha}(\meas{Q}_{t}: \meas{Q}) + 2 \gamma \cdot \langle g_{t}, \meas{Q} \rangle \right) - \int a(z) \meas{Q}(z) \dmeas{}z + b \left( 1 - \int \meas{Q}(z) \dmeas{}z \right)
    \end{equation*}
    
    We can now consider two cases.
    
    \textbf{\( \bullet \quad \max\left\{ 0, \frac{\rho}{1+\rho} \cdot (D_{\alpha}(\meas{P} : \meas{Q}) - \varepsilon)\right\} = \frac{\rho}{1+\rho} \cdot (D_{\alpha}(\meas{P} : \meas{Q}) - \varepsilon) \).}
    
    In this case, the first order optimality condition becomes,
    \begin{align*}
        0 
        &= \frac{\rho}{1+\rho} \cdot \frac{\partial}{\partial \meas{Q}(z)} \left( D_{\alpha}(\meas{P} : \meas{Q}) \right) + \frac{1}{1+\rho} \cdot \frac{\partial}{\partial \meas{Q}(z)} \left( D_{\alpha}(\meas{Q}_{t}: \meas{Q}) \right) + \frac{2 \gamma}{1+\rho}\cdot \frac{\partial}{\partial \meas{Q}(z)} \left(\langle g_{t}, \meas{Q} \rangle\right) - a(z) - b \\
        &= \frac{\rho}{1+\rho} \cdot \varphi^{\prime}_{\alpha}\left( \frac{\meas{Q}(z)}{\meas{P}(z)}\right) + \frac{1}{1+\rho} \cdot \varphi^{\prime}_{\alpha}\left( \frac{\meas{Q}(z)}{\meas{Q}_{t}(z)}\right) + \frac{2 \gamma}{1+\rho}\cdot g_{t}(z) - a(z) - b \\
        &= \frac{2}{\alpha-1} \cdot \frac{\rho}{1+\rho} \cdot \psi_{\alpha}\left( \frac{\meas{P}(z)}{\meas{Q}(z)}\right) + \frac{2}{\alpha-1} \cdot \frac{1}{1+\rho} \cdot \psi_{\alpha}\left( \frac{\meas{Q}_{t}(z)}{\meas{Q}(z)}\right) + \frac{2 \gamma}{1+\rho}\cdot g_{t}(z) - a(z) - b,
    \end{align*}
    following from \cref{sec:pf_opt_amicable_dist}.
    
    \todo{Need to ensure that the LHS is non-zero to divide across. Proof by contradiction. Need a lemma to state that the generalized average of non-simplex-boundary distributions is also not on the boundary.}
    Thus we have,
    \begin{align*}
        &\frac{\alpha-1}{2} \cdot \left( \frac{2 \gamma}{1+\rho}\cdot a(z) + b - g_{t}(z) \right) = \frac{\rho}{1+\rho} \cdot \psi_{\alpha}\left( \frac{\meas{P}(z)}{\meas{Q}(z)}\right) + \frac{1}{1+\rho} \cdot \psi_{\alpha}\left( \frac{\meas{Q}_{t}(z)}{\meas{Q}(z)}\right)  \\
        \iff & \frac{\alpha-1}{2} \cdot \left( \frac{2 \gamma}{1+\rho}\cdot a(z) + b - g_{t}(z) \right) = \frac{\rho}{1+\rho} \cdot \frac{\psi_{\alpha}(\meas{P}(z))}{\psi_{\alpha}(\meas{Q}(z))} + \frac{1}{1+\rho} \cdot \frac{\psi_{\alpha}(\meas{Q}_{t}(z))}{\psi_{\alpha}(\meas{Q}(z))} \\
        \iff & \frac{\alpha-1}{2} \cdot \left( \frac{2 \gamma}{1+\rho}\cdot a(z) + b - g_{t}(z) \right) = \frac{\frac{\rho}{1+\rho} \cdot {\psi_{\alpha}(\meas{P}(z))} + \frac{1}{1+\rho} \cdot {\psi_{\alpha}(\meas{Q}_{t}(z))}}{\psi_{\alpha}(\meas{Q}(z))} \\
        \iff & {\psi_{\alpha}(\meas{Q}(z))} = \left(\frac{\rho}{1+\rho} \cdot {\psi_{-\alpha}(\meas{P}(z))} + \frac{1}{1+\rho} \cdot {\psi_{-\alpha}(\meas{Q}_{t}(z))}\right) \cdot \frac{1}{\frac{\alpha-1}{2} \cdot \left( a(z) + b -\frac{2 \gamma}{1+\rho}\cdot g_{t}(z) \right)} \\
        \iff & \meas{Q}(z) = \psi_{\alpha}^{-1}\left(\frac{\rho}{1+\rho} \cdot {\psi_{\alpha}(\meas{P}(z))} + \frac{1}{1+\rho} \cdot {\psi_{\alpha}(\meas{Q}_{t}(z))}\right) \cdot \psi^{-1}_{\alpha}\left(\frac{1}{\frac{\alpha-1}{2} \cdot \left( a(z) + b -\frac{2 \gamma}{1+\rho}\cdot g_{t}(z) \right)}\right) \\
%        \iff & \meas{Q}(z) = c_{\alpha} \cdot \psi_{\alpha}^{-1}\left(\frac{\rho}{1+\rho} \cdot {\psi_{\alpha}(\meas{P}(z))} + \frac{1}{1+\rho} \cdot {\psi_{\alpha}(\meas{Q}_{t}(z))}\right) \cdot \frac{1}{\psi^{-1}_{\alpha}\left( a(z) + b -\frac{2 \gamma}{1+\rho}\cdot g_{t}(z)\right)} \\
        \iff & \meas{Q}(z) = m_{\alpha}\left[\meas{P}, \meas{Q}_{t}; \frac{\rho}{1 + \rho}\right](z) \cdot \psi^{-1}_{\alpha}\left(\frac{1}{\frac{\alpha-1}{2} \cdot \left( a(z) + b -\frac{2 \gamma}{1+\rho}\cdot g_{t}(z) \right)}\right).
    \end{align*}
    
    \textbf{\( \bullet \quad \max\left\{ 0, \frac{\rho}{1+\rho} \cdot (D_{\alpha}(\meas{P} : \meas{Q}) - \varepsilon)\right\} = 0 \).}
    
    This case follow similarly, which ends up being equivalent to the above case where \( \rho = 0 \):
    \begin{align*}
        \meas{Q}(z)
        &= \meas{Q}_{t}(z) \cdot \psi^{-1}_{\alpha}\left(\frac{1}{\frac{\alpha-1}{2} \cdot \left( a(z) + b -{2 \gamma}\cdot g_{t}(z) \right)}\right) \\
        &= m_{\alpha}\left[\meas{P}, \meas{Q}_{t}; \frac{\rho}{1 + \rho}\right](z) \cdot \psi^{-1}_{\alpha}\left(\frac{1}{\frac{\alpha-1}{2} \cdot \left( a(z) + b -\frac{2 \gamma}{1+\rho}\cdot g_{t}(z) \right)}\right).
    \end{align*}
\end{proof}

\todo{Change to \( \alpha < -1 \)}

For corollary, suppose that \( \alpha > 1 \).

% From prime feasibility, we require \( \meas{Q}(z) \geq 0 \).

It follows that as \( \alpha > 1 \) that \( c_{\alpha} > 0 \).

Suppose that \( \meas{Q}_{t} \) is not on the simplex boundary. Thus the averaging is also not on the boundary.
Note that \( \frac{1}{\psi^{-1}_{\alpha}(v)} \neq 0 \) for any \( v \in \Re \) when \( \alpha > 1 \). As a result, \( \meas{Q}(z) \neq 0 \).
Hence by complementary slackness, \( \alpha(z) = 0 \).

Further note that by prime feasibility, we also need \( \psi^{-1}_{\alpha}\left( b - \frac{2 \gamma}{1+\rho}\cdot g_{t}(z)\right) \geq 0 \). \( \psi^{-1}_{\alpha} \) will produce either an odd or even function with \( \alpha > 1 \). When it is odd, we require \( b - \frac{2 \gamma}{1+\rho} \cdot g_{t}(z) > 0 \) (otherwise the LHS is negative). When it is even, we may possibly have possible solutions for \( b \). However, we can restrict to be a unique solution by also restricting \( b - \frac{2 \gamma}{1+\rho} \cdot g_{t}(z) > 0 \).

Thus by examining the other prime feasibility condition, we can solve the following
\begin{align*}
    a(z) &= 0 \\
    1 &= c_{\alpha} \cdot \int m_{-\alpha}\left[\meas{P}, \meas{Q}_{t}; \frac{\rho}{1 + \rho}\right](z) \cdot \frac{1}{\psi^{-1}_{-\alpha}\left( b - \frac{2 \gamma}{1+\rho}\cdot g_{t}(z) \right)} \dmeas{}z\\
    b &> \frac{2 \gamma}{1+\rho}\cdot g_{t}(z).
\end{align*}

\begin{align*}
    1 &= c_{\alpha} \cdot \int \meas{P}(z) \cdot f\left( b - \frac{2 \gamma}{1+\rho}\cdot g_{t}(z) \right) \dmeas{}z \\
    b &> \frac{2 \gamma}{1+\rho}\cdot g_{t}(z).
\end{align*}
