# Supplementary material for: Rejection via Learning Density Ratios
Source: arXiv:2405.18686 source file (2025-05-08)
Supplement: Supplementary file 3 [file proof-adv-grad.tex]

\section{Proof of \cref{thm:adv_grad}}
\label{sec:pf_adv_grad}

\begin{proof}
    \begin{align*}
        &\grad_{\theta} \left( L(\meas{Q}_{\theta}) + \lambda \cdot (D_{\varphi}(\meas{P} : \meas{Q}_{\theta}) - \varepsilon) \right)\\
        &=
        \int_{\mathcal{X}} \grad_{\theta} \meas{Q}_{\theta}(\X) \cdot [\grad_{\meas{Q}}L(\meas{Q}_{\theta})](\X) + \lambda \cdot \grad_{\theta} \meas{Q}_{\theta}(\X) \cdot (\varphi^{\prime})^{-1}\left(\frac{\meas{Q}_{\theta}(\X)}{\meas{P}(\X)}\right)\\
        &=
        \int_{\mathcal{X}} \grad_{\theta} \meas{Q}_{\theta}(\X) \cdot \left( [\grad_{\meas{Q}}L(\meas{Q}_{\theta})](\X) + \lambda \cdot (\varphi^{\prime})^{-1}\left(\frac{\meas{Q}_{\theta}(\X)}{\meas{P}(\X)}\right)\right)\\
        &=
        \int_{\mathcal{X}} \meas{Q}_{\theta}(\X) \cdot \grad_{\theta} \log \meas{Q}_{\theta}(\X) \cdot \left( [\grad_{\meas{Q}}L(\meas{Q}_{\theta})](\X) + \lambda \cdot (\varphi^{\prime})^{-1}\left(\frac{\meas{Q}_{\theta}(\X)}{\meas{P}(\X)}\right)\right)\\
        &=
        \expect_{\meas{P}} \left[ \frac{\meas{Q}_{\theta}(\X)}{\meas{P}(\X)} \cdot \grad_{\theta} \log \meas{Q}_{\theta}(\X) \cdot \left( [\grad_{\meas{Q}}L(\meas{Q}_{\theta})](\X) + \lambda \cdot (\varphi^{\prime})^{-1}\left(\frac{\meas{Q}_{\theta}(\X)}{\meas{P}(\X)}\right)\right)\right].
    \end{align*}
\end{proof}
