# Supplementary material for: Rejection via Learning Density Ratios
Source: arXiv:2405.18686 source file (2025-05-08)
Supplement: Supplementary file 4 [file proof-bounded-lm.tex]

\section{Proof of \cref{prop:bounded_lm}}
\label{sec:pf_bounded_lm}

\begin{proof}
    \( D_{\alpha}(\meas{P} : \meas{Q}) \) is convex \wrt \( \meas{Q} \) due to it being a \( \varphi \)-divergence. Furthermore, it has a unique minimum at \( \meas{Q} = \meas{P} \). As such, \( \Vert \grad_{\meas{Q}} D_{\alpha}(\meas{Q} : \meas{P}) \Vert > 0 \) for \( \meas{Q} \neq \meas{P} \).
    
    Let \( c = \inf \left\{ \Vert \grad_{\meas{Q}} D_{\alpha}(\meas{P} : \meas{Q}) \Vert : \meas{Q} \in \mathcal{D}(\mathcal{Z}), D_{\alpha}(\meas{P} : \meas{Q}) > \varepsilon \right\} \). Given the above, \( c > 0 \) whenever \( \varepsilon > 0 \).
    
    Taking \( \lambda_{c} > \frac{M}{c} \), then \( D_{\alpha}(\meas{P} : \meas{Q}) > \varepsilon \) implies that \( 0 \not \in \partial_{\meas{Q}} \left( f(\meas{Q}; \vartheta) + \min\left\{ 0, \lambda_{c} \cdot \left( \varepsilon - D_{\alpha}(\meas{P} : \meas{Q}) \right) \right\} \right) \).
    
    Thus taking \( \lambda_{c} > \frac{M}{c} \), an optimal solution to \cref{eq:dro_dist_clip} must have \( D_{\alpha}(\meas{P} : \meas{Q}) < \varepsilon \). Noting that \( \min\left\{ 0, \lambda_{c} \cdot \left( \varepsilon - D_{\alpha}(\meas{P} : \meas{Q}) \right) \right\} = 0 \) when \( D_{\alpha}(\meas{P} : \meas{Q}) < \varepsilon \), an optimal distribution \( \meas{Q}^{\star} \) must minimize \( f(\meas{Q}; \vartheta) \) with \( D_{\alpha}(\meas{P} : \meas{Q}) < \varepsilon \), \ie, the constrained problem.
\end{proof}
